# Supplementary material for: Sketch-MoMa: Teleoperation for Mobile Manipulator via Interpretation of Hand-Drawn Sketches
Source: arXiv:2412.19153 source file (2026-11-06)
Supplement: Supplementary file 1 [file 6_appendix.tex]

\section*{APPENDIX}
\subsection{Bounding Box Composition with Sketches for Object Detection.}
\label{apx:object_detection}
\subsection{Path specification with Sketches.}
\label{apx:path}
\subsection{Flow of User Machine Interaction via 2D Interface.}
\label{apx:ui_flow}
\subsection{Text Prompts for Baselines.}
\label{apx:baseline_prompts}
\subsection{Additional Task Validation with Words}
\label{apx:pull-push-word}
\subsection{Whole Prompt for Sketch Interpretation.}
\label{apx:prompt}
